# Supplementary material for: PINCH: An Adversarial Extraction Attack Framework for Deep Learning Models
Source: arXiv:2209.06300 source file (2023-01-31)
Supplement: Supplementary file 1 [file Additional-Info.tex]

Dataset Complexity
- We now have a way of measuring the complexity of the datasets. CSG.

- Plot relationship of dataset complexity against average fidelity.

Architecture Complexity
- Relationship between number of model parameters vs fidelity + MAdd vs Fidelity

Equivalency
- Layer noise. Analysing sensitive layers within a model. Comparing most sensitive layers + shape. Why does that matter. Implication.

- Applied a distillation technique on a target and a stolen model of the same arch and dataset. Distilled into a 5 layer CNN.

    - Measured noise of sensitive layers between target distilled and stolen distilled models.

    - PWCCA between distilled models.
